# Supplementary material for: Matching 2D Images in 3D: Metric Relative Pose from Metric Correspondences
Source: arXiv:2404.06337 source file (2024-04-09)
Supplement: Supplementary file 1 [file MickeyOverlap.tex]

\begin{table*}[t]
\footnotesize
\begin{center}
\begin{tabular}{l l c l c c l c c l c c c}
\multicolumn{13}{c}{\textbf{MapFree Dataset}}\\ 
\cline{1-13}
\noalign{\smallskip}
\cline{1-13}
\noalign{\smallskip}
\multicolumn{4}{c}{} & \multicolumn{2}{c}{VCRE ($<$ 90px)} & \multicolumn{1}{c}{} & \multicolumn{2}{c}{Pose Err ($<$ 25cm, 5\textdegree)} & \multicolumn{1}{c}{} & \multicolumn{3}{c}{Median Errors}\\ 
\cline{5-6} \cline{8-9}  \cline{11-13} \noalign{\smallskip}
\multicolumn{4}{c}{} & \multicolumn{1}{c}{AUC} & \multicolumn{1}{c}{Prec. (\%)} & \multicolumn{1}{c}{} & \multicolumn{1}{c}{AUC} & \multicolumn{1}{c}{Prec. (\%)} & \multicolumn{1}{c}{} & \multicolumn{1}{c}{Rep. (px)} & \multicolumn{1}{c}{Trans. (m)} & \multicolumn{1}{c}{Rot. (\textdegree)} \\ 
\cline{1-13}
\noalign{\smallskip}
&& SIFT - DPT && 0.50 & 25.0 && 0.25 & 10.3 && 222.8 & 2.93 & 61.4\\
&& SiLK - DPT && x & x && x & x && x & x & x\\
\cline{1-13}
\noalign{\smallskip}
% \textbf{Depth Supervision} &&& \\
\multirow{10}{*}{\rotText{\rotatebox[origin=c]{90}{\textbf{Depth + Overlap + Pose}}}}
\multirow{10}{*}{\rotText{\rotatebox[origin=c]{90}{\textbf{Supervision}}}}
&& \textbf{Sparse Features} &&& \\
\cline{3-3} \noalign{\smallskip}
&& DISK - DPT && x & x && x & x && x & x & x\\
&& DeDoDe - DPT && x & x && x & x && x & x & x\\
&& SuperPoint - SuperGlue - DPT  && 0.60 & 36.1 && 0.35 & 16.8 && 160.3 & 1.88 & 25.4\\
&& DISK - LightGlue - DPT && x & x && x & x && x & x & x\\
\noalign{\smallskip}
&& \textbf{Dense Features} &&& \\
\cline{3-3} \noalign{\smallskip}
&& LoFTR - DPT  && 0.61 &34.7 && 0.35 & 15.4 && 167.6 & 1.98 & 30.5\\
&& ASpanFormer - DPT && x & x && x & x && x & x & x\\
&& ROMA - DPT && 0.67 & 45.6 && \textbf{0.41} & \textbf{22.8} && 128.8 & \textbf{1.23} & \textbf{11.1}\\
\cline{1-13}
\noalign{\smallskip}
\noalign{\smallskip}
\multirow{4}{*}{\rotText{\rotatebox[origin=c]{90}{\textbf{Pose}}}}
\multirow{1}{*}{\rotText{\rotatebox[origin=c]{90}{\textbf{Supervision}}}}
&& RPR [R($\alpha, \beta, \gamma$) + s $\cdot$t($\theta, \omega$)] && 0.35 & 35.4 && 0.10 & 10.5 && 166.3 & 1.83 & 23.2\\
&& RPR [3D-3D] && 0.39 & 38.7 && 0.06 & 6.0 && 148.7 & 1.69 & 22.9\\
&& RPR [(R(6D) + t] && 0.40 & 40.2 && 0.06 & 6.0 && 147.1 & 1.68 & 22.5\\
&& MicKey  && \textbf{0.74} & \textbf{49.2} && 0.28 & 12.0 && \textbf{126.9} & 1.59 & 25.9\\
\cdashline{2-13}\noalign{\smallskip}
&& MicKey w/ Overlap - Medium && 0.75 & 49.2 && 0.33 & 13.3 && 129.4 & 1.65 & 27.2 \\
&& MicKey w/ Overlap - Easy && 0.70 & 42.1 && 0.36 & 14.6 && 141.3 & 2.08 & 35.5 \\
\end{tabular}
\end{center}
\vspace{-2em}
\normalsize
\caption{\textbf{Relative pose evaluation on MapFree}. }
\label{tab:mapfree_main_table}
\end{table*}
