# Supplementary material for: Matching 2D Images in 3D: Metric Relative Pose from Metric Correspondences
Source: arXiv:2404.06337 source file (2024-04-09)
Supplement: Supplementary file 2 [file depth_ablation_metrics.tex]

\begin{table}[t]
\footnotesize
\begin{center}
\begin{tabular}{cccc}
\multicolumn{1}{c}{\textbf{AUC / Prec. (VCRE)}} & \multicolumn{1}{c}{DPT [58]} & \multicolumn{1}{c}{ZoeDepth} & \multicolumn{1}{c}{\textbf{\ours's Depth}}\\ 
\hline \noalign{\smallskip}
RoMa [22] & 0.67 / 45.6 & 0.67 / 47.2 & \textbf{0.73} / \textbf{52.4}\\
\end{tabular}
\end{center}
\vspace{-1.8em}
\normalsize
\caption{\textbf{RoMa+depth} (Map-free dataset). \ours: 0.75/49.2 }
\label{tab:ablation_roma_depth}
% \vspace{-0.8em}
\end{table}

\begin{table}[t]
\footnotesize
\begin{center}
\begin{tabular}{ccccc}
\multicolumn{1}{c}{\textbf{ScanNet}} & \multicolumn{1}{c}{$\delta_1$ / $\delta_2$ / $\delta_3$ $\uparrow$} & \multicolumn{1}{c}{REL $\downarrow$} & \multicolumn{1}{c}{RMSE $\downarrow$} & \multicolumn{1}{c}{$\text{log}_{10}$ $\downarrow$} \\ 
\hline \noalign{\smallskip}
DPT [58] & 0.72 / 0.91 / 0.97 & 0.21 & 0.38 & 0.08 \\
PlaneRCNN [46] & 0.75 / 0.93 / \underline{0.98} & 0.18 & 0.37 & \underline{0.07} \\
ZoeDepth & \underline{0.79} / \underline{0.94} / \underline{0.98} & 0.17 & \textbf{0.33} & \underline{0.07} \\
\textbf{\ours} & \underline{0.79} / \textbf{0.95} / \underline{0.98} & \underline{0.16} & 0.37 & \textbf{0.06} \\
\textbf{\ours-Sc} & \textbf{0.80} / \textbf{0.95} / \textbf{0.99} & \textbf{0.15} & \underline{0.35} & \textbf{0.06} \\
\end{tabular}
\end{center}
\vspace{-1.8em}
\normalsize
\caption{\textbf{Monodepth metrics} in the ScanNet dataset.}
\label{tab:monodepth_scannet}
% \vspace{-0.8em}
\end{table}
